# Supplementary material for: Fine-Tuning on Diverse Reasoning Chains Drives Within-Inference CoT Refinement in LLMs
Source: arXiv:2407.03181 source file (2025-05-27)
Supplement: Supplementary file 1 [file performance_across_k.tex]

\Cref{fig:k_progression} shows the performance gains of \texttt{DCoT@k} against \texttt{DCoT@1}.
